# Supplementary material for: Stubborn Set Reduction for Two-Player Reachability Games
Source: arXiv:1912.09875 source file (2021-03-17)
Supplement: Supplementary file 1 [file appendix.tex]

\section{Proof of Lemma~\ref{lemma:depth}}
\begin{proof}
	(\ref{stratA}):
	Due to $\ltslabels_1$ and $\ltslabels_2$ being finite as well as any $\lts$ being deterministic we have every state $s \in \ltsstates$ is finitely branching.
	Since $s$ is a winning state for player $1$ in $\lts$ every path leads to a goal state in a finite number of actions.
	Therefore the tree induced by all paths starting from $s$ and where the leafs are the first occurring goal state is a finite tree, and $n$ exists.

	(\ref{stratB}):
	Let $n$ be the depth of $\sigma$ at $s$ in $\lts$ and $\pi \in \maxpaths_{\lts,\sigma}(s)$ be any path subject to $\sigma$ s.t. $\pi_0 \rtrans[a] \pi_1$ and $a \in \stratnext{\sigma}{s}$.
	If $\pi_n \in \goal$ and for all $0 \leq j < n$ we have $\pi_j \notin \goal$ then the depth of $\sigma$ at $\pi_1$ in $\lts$ is $n-1$.
	Otherwise there must exist some other run $\pi' \in \maxpaths_{\lts,\sigma}(s)$ s.t. $\pi'_1 = \pi_1$ and there exists $m \in \mathbb{N}^0$ s.t. $\pi'_m \in \goal$, $m < n$, and for all $0 \leq j < m$ we have $\pi_j \notin \goal$.
	Then $m-1$ is the depth of $\sigma$ at $\pi_1$ in $\lts$.
\end{proof}

\section{Proof of Lemma~\ref{lemma:early-termination}}
\begin{proof}
	Assume that there exists $w = a_1 \cdots a_n \in \ltslabels^*$ s.t. $s \rtrans[w] s'$ and $s' \in \goal$.
	If $w \in \overline{\reduction(s)}^*$ then by Condition~\ref{rule:reach} we must have $s' \notin \goal$, however this contradicts our assumption.
	Therefore there must exist an action that occurs in $w$ that is in the stubborn set of $s$.
	Let $a_i \in \reduction(s)$ be the first of such an action s.t. for all $1 \leq j < i$ we have $a_j \notin \reduction(s)$.
	Clearly we have $a_1 \cdots a_j \in \overline{\reduction(s)}^*$ and by Condition~\ref{rule:stub} we have $a_i \in \reduction(s) \cap \en(s)$.
\end{proof}

\section{Proof of Lemma~\ref{lemma1}}
\begin{proof}
	Assume that $s \in \ltsstates$ is a winning state for player $1$ in $\lts$.
	By definition we have that there exists $\sigma$ s.t. for all $\pi \in \maxpaths_{\lts,\sigma}(s)$ there exists a position $i$ s.t. $\pi_i \in \goal$.

	We prove by induction $\mathit{IH}(n)$: If $s$ is a winning state for player $1$ in $\lts$ with a strategy with a depth of $n$ then $s$ is a winning state for player $1$ in $\lts_{\reduction}$.

	\emph{Base step}.
	Let $n = 0$.
	Then since $n$ is the depth at $s$ in $\lts$ we must have $s \in \goal$, $s$ is trivially a winning state for player $1$ also in $\lts_{\reduction}$, and the induction hypothesis holds.

	\emph{Induction step}.
	Let $n > 0$.
	There are three cases: (1) $\en_1(s) \neq \emptyset$ and $\en_2(s) \neq \emptyset$, (2) $\en_2(s) = \emptyset$, and (3)  $\en_1(s) = \emptyset$.
	A deadlock at $s$, i.e. $\en(s) = \emptyset$, cannot be the case otherwise we have $n = 0$.

	Case (1): $\en_1(s) \neq \emptyset$ and $\en_2(s) \neq \emptyset$.
	Assume $s$ is a winning state for player $1$ in $\lts$ with a strategy $\sigma$ with a depth of $n$.
	We want to show there exists a strategy $\sigma'$ s.t. $s$ is a winning state for player $1$ in $\lts_{\reduction}$ with $\sigma'$.
	Since $s$ is a winning state for player $1$ in $\lts$ with $\sigma$ if $s \rtrans[a] s'$ where $a \in \stratnext{\sigma}{s}$ then $s'$ is a winning state for player $1$ in $\lts$ with $m < n$ as the depth of $\sigma$ at $s'$ in $\lts$, following property~\ref{stratB} in Lemma~\ref{lemma:depth}.
	By the induction hypothesis $s'$ is a winning state for player $1$ in $\lts_{\reduction}$.
	By Condition~\ref{rule:stub-init} we know $\en_1(s) \subseteq \reduction(s)$ implying that $\sigma(s) \in \reduction(s)$.
	Player $1$ can therefore choose the same action proposed in the original game s.t. $\sigma'(s) = \sigma(s)$ and $s$ is a winning state for player $1$ in $\lts_{\reduction}$.

	Case (2): $\en_2(s) = \emptyset$.
	Assume $s$ is a winning state for player $1$ in $\lts$ with a strategy $\sigma$ with a depth of $n$.
	We want to show there exists a strategy $\sigma'$ s.t. $s$ is a winning state for player $1$ in $\lts_{\reduction}$ with $\sigma'$.
	Let $\pi \in \maxpaths_{\lts,\sigma}(s)$ be any run and $\pi_0 = s$.
	Since $s$ is a winning state for player $1$ in $\lts$ with $\sigma$ we know there exists a $m \leq n$ s.t. $\pi_0 \rtrans[a_1] \pi_1 \rtrans[a_2] \cdots \rtrans[a_m] \pi_m$ and $\pi_m \in \goal$.
	Let $w = a_1 \cdots a_m$.
	We start by showing that there exists $1 \leq i \leq m$ s.t. $a_i \in \reduction(s)$.
	Assume that $w \in \overline{\reduction(s)}^*$ is true.
	Then we have $\pi_m \notin \goal$ due to Condition~\ref{rule:reach}, a contradiction.
	Therefore there must exist $1 \leq i \leq m$ s.t. $a_i \in \reduction(s)$.
	Let $i$ be minimal in the sense that for all $1 \leq j < i$ we have $a_j \notin \reduction(s)$.
	We can then divide $w$ s.t. $w = va_iu$, $v \in \overline{\reduction(s)}^*$ and we have $s \rtrans[a_i] s'_0 \rtrans[v] \pi_i \rtrans[u] \pi_m$ due to Condition~\ref{rule:stub} as well as $s \rtrans[a_i][\reduction] s'_0$.
	There are two subcases: (2.1) $a_i \in \safe{s}$ and (2.2) $a_i \notin \safe{s}$.
	\begin{itemize}
		\item Case (2.1): $a_i \in \safe{s}$:
		For all $1 \leq j < i$ we have $\en_2(\pi_j) = \emptyset$ due to $i$ being minimal and Condition~\ref{rule:game-1}.
		From that, if $a_i \in \safe{s}$ then for all all intermediate states in $s \rtrans[a_iv] \pi_i$ we only have player $1$ states otherwise $a_i$ is not a safe action due to the definition of safe actions.
		We have that $s'_0$ is a player $1$ state and there exists the sequence $v = a'_1 a'_2 \cdots a'_{i-1}$ s.t. $s'_0 \rtrans[a'_1] s'_1 \rtrans[a'_2] \cdots \rtrans[a'_{i-1}] \pi_i$ and for all $1 \leq k < i-1$ we have $\en_2(s'_k) = \emptyset$.
		Let $\sigma'$ be defined such that for all $0 \leq j < i-1$ we have $\sigma(s'_{j-1}) = a'_j$, and let $\sigma'$ from $\pi_i$ be defined as $\sigma$.
		Due to property~\ref{stratB} in Lemma~\ref{lemma:depth} the depth of $\sigma$ at $\pi_i$ in $\lts$ is at most $k \leq n-i$.
		Since $\lts$ is deterministic by following the strategy $\sigma'_1$ from $s'_0$ we always reach $\pi_i$ in $i-1$ actions.
		From this we can infer that the depth of $\sigma'_1$ at $s'_0$ in $\lts$ is at most $k+i-1$ which is clearly smaller than $n$.
		Therefore $s'_0$ is a winning state for player $1$ in $\lts$ with at most $k+i-1$ as the depth of $\sigma'$ at $s'_0$ in $\lts$.
		By the induction hypothesis $s'_0$ is a winning state for player $1$ in $\lts_{\reduction}$.
		Player $1$ can then choose $a_i$ in the reduced game such that $\sigma'(s) = a_i$ and $s$ is a winning state for player $1$ in $\lts_{\reduction}$.
		\item Case (2.2): $a_i \notin \safe{s}$:
		Since $a_i \notin \safe{s}$ we have $\reduction(s) \cap \en_1(s) \nsubseteq \safe{s}$ and $\en_1(s) \subseteq \reduction(s)$ by Condition~\ref{rule:safe}.
		If $s \rtrans[\sigma(s)] s'$ then $s'$ is a winning state for player $1$ in $\lts$ with $m < n$ as the depth of $\sigma$ at $s'$ in $\lts$, following property~\ref{stratB} in Lemma~\ref{lemma:depth}.
		By the induction hypothesis $s'$ is a winning state for player $1$ in $\lts_{\reduction}$.
		Player $1$ can choose the same action proposed in the original game such that $\sigma'(s) = \sigma(s)$ and $s$ is a winning state for player $1$ in $\lts_{\reduction}$.
	\end{itemize}

	Case (3): $\en_1(s) = \emptyset$.
	Assume $s$ is a winning state for player $1$ in $\lts$ with $\sigma$ as the winning strategy.
	We want to show there exists a strategy $\sigma'$ s.t. $s$ is a winning state for player $1$ in $\lts_{\reduction}$ with $\sigma'$.
	Since $\en_1(s) = \emptyset$ we have $\sigma(s) = \sigma'(s) = \bot$ by the definition of strategies.
	We have from the definition of a winning strategy no matter what action player $2$ chooses the resulting state is a winning state for player $1$.
	What remains to be shown is that at least one enabled player $2$ action is included in $\reduction(s)$.
	From the case we have $\en_2(s) \neq \emptyset$ and due to Condition~\ref{rule:dead} we have that there exists $a \in \en_2(s) \cap \reduction(s)$ s.t. $s \rtrans[a][\reduction] s'$, and we are done.
\end{proof}

\section{Proof of Lemma~\ref{lemma2}}
\begin{proof}
	Assume that $s \in \ltsstates$ is a winning state for player $1$ in $\lts_{\reduction}$.
	By definition we have that there exists $\sigma$ s.t. for all $\pi \in \maxpaths_{\lts_{\reduction},\sigma}(s)$ there exists a position $i$ s.t. $\pi_i \in \goal$.
	Let $\sigma$ be fixed for the remainder of the proof.
	Let $n$ be the depth of $\sigma$ at $s$ in $\lts_{\reduction}$.

	We proceed by induction on $n$ for the induction hypothesis $\mathit{IH}(n)$: If $s$ is a winning state for player $1$ in $\lts_{\reduction}$ with a strategy with a depth of $n$ then $s$ is a winning state for player $1$ in $\lts$.

	\emph{Base step}.
	If $n = 0$ then since $n$ is the depth at $s$ in $\lts_{\reduction}$ we must have $s \in \goal$, $s$ is trivially a winning state for player $1$ also in $\lts$, and the induction hypothesis holds.

	\emph{Induction step}.
	Let $n > 0$.
	There are three cases: (1) $\en_1(s) \cap \reduction(s) \neq \emptyset$ and $\en_2(s) \cap \reduction(s) \neq \emptyset$, (2) $\en_2(s) \cap \reduction(s) = \emptyset$, and (3)  $\en_1(s) \cap \reduction(s) = \emptyset$.
	A deadlock at $s$, i.e. $\en(s) = \emptyset$, cannot be the case otherwise we have $n = 0$.
	A deadlock in $\lts_{\reduction}$ at, i.e. $\en(s) \cap \reduction(s) = \emptyset$ $s$ cannot be the case either otherwise we have $n = 0$.

	Case (1): $\en_1(s) \cap \reduction(s) \neq \emptyset$ and $\en_2(s) \cap \reduction(s) \neq \emptyset$.
	Assume $s$ is a winning state for player $1$ in $\lts_{\reduction}$ with a strategy $\sigma$ with a depth of $n$.
	We want to show there exists a strategy $\sigma'$ s.t. $s$ is a winning state for player $1$ in $\lts$ with $\sigma'$.
	Since $s$ is a winning state for player $1$ in $\lts_{\reduction}$ with $\sigma$ if $s \rtrans[\sigma(s)][\reduction] s'$ or $s \rtrans[a][\reduction] s'$ where $a \in \en_2(s) \cap \reduction(s)$ then $s'$ is a winning state for player $1$ in $\lts_{\reduction}$ with $m < n$ as the depth of $\sigma$ at $s'$ in $\lts_{\reduction}$, following property~\ref{stratB} in Lemma~\ref{lemma:depth}.
	By the induction hypothesis $s'$ is a winning state for player $1$ in $\lts$.
	Since $s$ is a mixed state in $\lts_{\reduction}$ then $s$ must also be a mixed state in $\lts$ due to $\rtrans[][\reduction] \subseteq \ltsedges$ from the definition of a reduced game and so $s \rtrans[\sigma(s)] s'$.
	Therefore player $1$ can choose the same action proposed in the reduced game such that $\sigma'(s) = \sigma(s)$.
	Furthermore we have $\en_2(s) \cap \reduction(s) = \en_2(s)$ fron Condition~\ref{rule:stub-init}.
	From this we can conclude that $s$ is a winning state for player $1$ in $\lts$ with strategy $\sigma'$.

	Case (2): $\en_2(s) \cap \reduction(s) = \emptyset$.
	Assume $s$ is a winning state for player $1$ in $\lts_{\reduction}$ with a strategy $\sigma$ with a depth of $n$.
	We want to show there exists a strategy $\sigma'$ s.t. $s$ is a winning state for player $1$ in $\lts$ with $\sigma'$.
	Since $s$ is a winning state for player $1$ in $\lts_{\reduction}$ with $\sigma$ we have $s \rtrans[\sigma(s)][\reduction] s'$ and $s'$ is a winning state for player $1$ in $\lts_{\reduction}$ with $m < n$ as the depth of $\sigma$ at $s'$ in $\lts_{\reduction}$, following property~\ref{stratB} in Lemma~\ref{lemma:depth}.
	By the induction hypothesis $s'$ is a winning state for player $1$ in $\lts$.
	Trivially we have that $s \rtrans[\sigma(s)] s'$ since we have $\rtrans[][\reduction] \subseteq \ltsedges$ from the definition of a reduced game.
	Therefore player $1$ can choose the same action proposed in the reduced game $\sigma'(s) = \sigma(s)$.
	Next we want to show by contradiction that $s$ is a player $1$ state in $\lts$.
	Assume $\en_2(s) \neq \emptyset$, i.e. that $s$ is a mixed state in $\lts$.
	From this we can infer by Condition~\ref{rule:stub-init} that $\en(s) \subseteq \reduction(s)$ and $\en_2(s) \cap \reduction(s) \neq \emptyset$, which is a contradiction.
	Therefore we have $\en_2(s) = \emptyset$, i.e. $s$ is a player $1$ state also in $\lts$, and $s$ is a winning state for player $1$ in $\lts$ with strategy $\sigma'$.

	Case (3): $\en_1(s) \cap \reduction(s) = \emptyset$.
	Assume $s$ is a winning state for player $1$ in $\lts_{\reduction}$ with a strategy $\sigma$ with a depth of $n$.
	We want to show there exists a strategy $\sigma'$ s.t. $s$ is a winning state for player $1$ in $\lts$ with $\sigma'$.
	Since $\en_1(s) \cap \reduction(s) = \emptyset$ then we have $\sigma(s) = \bot$.
	Furthermore, we have $\en_1(s) = \emptyset$ since otherwise with Condition~\ref{rule:stub-init} we will be able to infer that $\en_1(s) \cap \reduction(s) \neq \emptyset$, which is a contradiction.
	Therefore, in any case we define $\sigma'(s) = \bot$ due to the definition of a strategy.
	Since $s$ is a winning state for player $1$ in $\lts_{\reduction}$ with $\sigma$ if $s \rtrans[a][\reduction] s'$ where $a \in \en_2(s) \cap \reduction(s)$ then $s'$ is a winning state for player $1$ in $\lts_{\reduction}$ with $m < n$ as the depth of $\sigma$ at $s'$ in $\lts_{\reduction}$, following property~\ref{stratB} in Lemma~\ref{lemma:depth}.
	By the induction hypothesis $s'$ is a winning state for player $1$ in $\lts$.

	What remains to be shown is that for all $a \in \en_2(s) \setminus \reduction(s)$ where $s \rtrans[a] s'$ that $s'$ is a winning state for player $1$ in $\lts$.
	We show by contradiction that this is the case.
	Assume there exists $\pi \in \maxpaths_{\lts}(s)$ s.t. $\pi_0 \rtrans[a_1] \pi_1$ and $a_1 \in \en_2(s) \setminus \reduction(s)$ and for all $i > 0$ we have $\pi_i \notin X$ and $\pi_1 \rtrans[a_2] \pi_2 \rtrans[a_3] \cdots$.
	There are two subcases: (3.1) for all $i > 0$ we have $a_i \in \ltslabels_2$ and (3.2) there exists a minimal $i > 1$ s.t. $a_i \in \ltslabels_1$.
	\begin{itemize}
		\item Case (3.1): For all $i > 0$ we have $a_i \in \ltslabels_2$:
		In this case we have another two subcases: (3.1.1) $\pathlen(\pi) = \infty$ and (3.1.2) $\en(\pi_{\pathlen(\pi)}) = \emptyset$.
		\begin{itemize}
			\item Case (3.1.1): $\pathlen(\pi) = \infty$:
%			In this case we have that there exists $w \in \ltslabels_2^{\omega}$ s.t. $s \rtrans[w]$, namely $w = a_1 a_2 \cdots$.
%			From we this we have that the antecedent of Condition~\ref{rule:cycle} is true, and we must have that $\en_2(s) \subseteq \reduction(s)$, implying that $a_1 \in \reduction(s)$.
%			However this is a contradiction since $a_1 \in \en_2(s) \setminus \reduction(s)$.
%			Therefore we have that $\pi$ does not exist.
			In this case we have that there exists $w \in \ltslabels_2^{\omega}$ s.t. $s \rtrans[w]$, namely $w = a_1 a_2 \cdots$.
			Let $a_{m+1}$ be the first action to occur in $w$ that also occurs infinitely often in $w$ s.t. $w = va_{m+1}u$, $v = a_1 \cdots a_{m}$, and $s \rtrans[v] s_m \rtrans[a_{m+1}u]$.
			Since the set of labels $\ltslabels$ is finite such an action must exist.
			We proceed by induction on the length $m$ to show that a path to $s_m$ is preserved with the induction hypothesis $\mathit{IH}(m)$: If there exists $w \in \ltslabels_2^*$ s.t. $|w| = m$ and $s \rtrans[w] s_m$ then there exists $w' \in \ltslabels_2^*$ s.t. $s \rtrans[w'][\reduction] s_m$.
			\emph{Base step}. Trivial for $m = 0$.
			\emph{Induction step}. Let $m > 0$.
			We have already assumed that $s_m$ can be reached from $s$ in $m$ actions using only player $2$ actions in $\lts$ with the sequence $v$.
			We want to show by contradiction that there exists a minimal $1 \leq j \leq m$ s.t. $a_j \in \reduction(s)$.
			By Condition~\ref{rule:cycle} we have $a_{m+1} \in \reduction(s)$.
			If $a_{m+1} \notin \en(s)$ and $v \in \overline{\reduction(s)}^*$ then this would contradict Condition~\ref{rule:stub}.
			Therefore, there must exist $1 \leq j \leq m$ s.t. $a_j \in \reduction(s)$.
			From this we can divide $v$ s.t. $v = v'a_ju'$ and $v' \in \overline{\reduction(s)}^*$.
			Then due to Condition~\ref{rule:stub} we have $s \rtrans[a_j] s'' \rtrans[v'u'] s_m$, $|v'u'| = m-1$, and $s \rtrans[a_j][\reduction] s''$.
			By the inner induction hypothesis we have there exists $w' \in \ltslabels_2^*$ s.t. $s'' \rtrans[w'][\reduction] s_m$ and $|w'| = m-1$.
			With $s \rtrans[a_j][\reduction] s''$ we have $s \rtrans[a_jw'] s_m$ and a path to $s_m$ is preserved.
			At $s_m$ we have $a_{m+1} \in \reduction(s_m)$ by Condition~\ref{rule:cycle}, and the same argument can be applied for each subsequent state and action in $w$, and an infinite path of player $2$ actions is preserved.
			Therefore, $s$ is a losing state for player $1$
			However this is a contradiction since $s$ is a winning state for player $1$ in $\lts_{\reduction}$.
			Therefore we have that $\pi$ does not exist.
			\item Case (3.1.2) $\en(\pi_{\pathlen(\pi)}) = \emptyset$:
			Let $w = a_1 \cdots a_{\pathlen(\pi)}$.
			To show the contradiction we will proceed by induction on the length $m = |w|$ with the induction hypothesis $\mathit{IH}(m)$: If there exists $w' = a_1' \cdots a_m' \in \ltslabels_2^*$ s.t. $s \rtrans[a_1'] s_1 \rtrans[a_2'] \cdots \rtrans[a_m'] s'$, $|w'| = m$, $\en(s') = \emptyset$, and for all $0 \leq k \leq m$ we have $\pi_k \notin \goal$ then $s$ is a winning state for player $2$ in $\lts_{\reduction}$.
			\emph{Base step}. Trivial for $m = 0$.
			\emph{Induction step}. Let $m > 0$.
			We have already assumed that a deadlock can be reached from $s$ in $m$ actions using only player $2$ actions in $\lts$ with the path $\pi$.
			We want to show by contradiction that there exists a minimal $1 \leq j \leq \pathlen(\pi)$ s.t. $a_j \in \reduction(s)$.
			Now assume that $w \in \overline{\reduction(s)}^*$.
			From Condition~\ref{rule:dead} we have that there exists $a \in \en_2(s) \cap \reduction(s)$ s.t. for all $w \in \overline{\reduction(s)}^*$ where $s \rtrans[w] s''$ we have $a \in \en_2(s'')$.
			From this we have $a \in \en_2(\pi_{\pathlen(\pi)})$, which is a contradiction.
			Therefore there must exist a minimal $1 \leq j \leq \pathlen(\pi)$ s.t. $a_j \in \reduction(s)$.
			From this we can divide $w$ s.t. $w = v a_j u$ and $v \in \overline{\reduction(s)}^*$.
			Then due to Condition~\ref{rule:stub} we have $s \rtrans[a_j] s'' \rtrans[vu] \pi_{\pathlen(\pi)}$, $|vu| = m-1$, and $s \rtrans[a_j][\reduction] s''$.
			We have $s'' \notin \goal$ since otherwise we would have $a_1 \in \reduction(s)$ by Condition~\ref{rule:reach}, which is a contradiction.
			By the inner induction hypothesis $s''$ is a winning state for player $2$ in $\lts_{\reduction}$.
			We already showed that $a_j \in \reduction(s)$ s.t. $s \rtrans[a_j][\reduction(s)] s''$.
			We therefore have that $s$ is a winning state for player $2$ in $\lts_{\reduction}$ since the path $\pi$ is preserved.
			However this is a contradiction since $s$ is a winning state for player $1$ in $\lts_{\reduction}$.
			Therefore we have that $\pi$ does not exist.
		\end{itemize}
		\item Case (3.2): There exists a minimal $i > 1$ s.t. $a_i \in \ltslabels_1$:
		Let $w = a_1 \cdots a_{i-1}$.
		To show the contradiction we will proceed by induction on $m = i-1$ with the induction hypothesis $\mathit{IH}(m)$: If there exists $w' \in \ltslabels_2^*$ s.t. $s \rtrans[w']$, $\pi_{i-1}$, $|w'| = m$, $\en(s) = \emptyset$, and for all $0 \leq k \leq m$ we have $\pi_k \notin \goal$ then $s$ is a winning state for player $2$ in $\lts_{\reduction}$.
		\emph{Base step}. Trivial for $m = 0$.
		\emph{Induction step}. Let $m > 0$.
		We have already assumed that $\pi_{i-1}$ can be reached from $s$ in $m$ steps using only player $2$ actions in $\lts$ with the path $\pi$.
		We want to show by contradiction that there exists a minimal $1 \leq j < i$ s.t. $a_j \in \reduction(s)$.
		Now assume that $w \in \overline{\reduction(s)}^*$.
		Then due to Condition~\ref{rule:game-2} we have $\en_1(\pi_{i-1}) = \emptyset$, which is a contradiction.
		Therefore there must exist a minimal $1 \leq j < i$ s.t. $a_j \in \reduction(s)$.
		From this we can divide $w$ s.t. $w = v a_j u$ and $v \in \overline{\reduction(s)}^*$.
		Then due to Condition~\ref{rule:stub} we have $s \rtrans[a_j] s'' \rtrans[vu] \pi_{i-1}$, $|vu| = m-1$, and $s \rtrans[a_j][\reduction] s''$.
		We have $s'' \notin \goal$ since otherwise we would have $a_1 \in \reduction(s)$ by Condition~\ref{rule:reach}, which is a contradiction.
		By the induction hypothesis $s''$ is a winning state for player $2$ in $\lts_{\reduction}$.
		We already showed that $a_j \in \reduction(s)$ s.t. $s \rtrans[a_j][\reduction(s)] s''$.
		We therefore have that $s$ is a winning state for player $2$ in $\lts_{\reduction}$ since the path $\pi$ is preserved.
		However this is a contradiction since $s$ is a winning state for player $1$ in $\lts_{\reduction}$.
		Therefore we have that $\pi$ does not exist.
	\end{itemize}
	We have showed in every case that $\pi$ cannot exist.
	Therefore for all $a \in \en_2(s) \setminus \reduction(s)$ where $s \rtrans[a] s'$ we have that $s'$ is a winning state for player $1$ in $\lts$.

	Finally, since we have showed that for all $a \in \en_2(s)$ where $s \rtrans[a] s'$ we have $s'$ is a winning state for player $1$ in $\lts$, then we can conclude that $s$ is a winning state for player $1$ in $\lts$.
\end{proof}

\section{Proof of Theorem~\ref{theorem:preservation-1}}
\begin{proof}
	Follows from Lemma~\ref{lemma1} and~\ref{lemma2}.
\end{proof}

\section{Proof of Theorem~\ref{theorem:preservation-2}}
\begin{proof}
	The proof of Theorem~\ref{theorem:preservation-2} follows the same approach as in Lemma~\ref{lemma1} and~\ref{lemma2}, with only Case 2 from Lemma~\ref{lemma1} receiving changes that makes the case easier.

	When the first action in the reduction $a_i \in \reduction(s)$ is swapped by Condition~\ref{rule:stub}, s.t. $s \rtrans[a_j] s' \rtrans[v] a_i$, we know $s'$ is a player $1$ state (as well as every intermediate state between $s'$ and $s_m$) otherwise $s' \rtrans[v] s_m$ is not possible since $v \in \ltslabels_1^*$.
	Therefore, whether $a_i$ is safe or not is not relevant, and $s'$ is a winning state for player $1$ in $\lts$.
\end{proof}

\section{Proof of Lemma~\ref{lemma:trans-safe}}
\begin{proof}
	Assume $\postincr{t} \cap \preset{T_2} = \emptyset$ and $\predecr{t} \cap \inhibpreset{T_2} = \emptyset$.
	We prove directly that $t$ is safe in $M$.
	Let 	$w \in (\transitions_1 \setminus \{ t \})^*$ s.t. $M \rtrans[w] M'$, $\en_2(M') = \emptyset$, and $M \rtrans[tw] M''$.
	The only difference between $M'$ and $M''$ is that $t$ is fired first and we have $M''(p') = M'(p') + \weights((t,p')) - \weights((p',t))$ for all $p \in \places$.
	Then for all $t' \in \transitions_2$ we have that there either exists $p \in \preset{t'}$ s.t. $M'(p) <\weights((p,t'))$, or there exists $p' \in \inhibpreset{t'}$ s.t. $M'(p') \geq \inhib((p',t'))$.
	In the first case, since $\postincr{t} \cap \preset{T_2} = \emptyset$, we must have $\weights((t,p)) \leq \weights((p,t))$ which implies $M''(p) \leq M'(p)$ and $t' \notin \en(M'')$.
	In the second case, since $\predecr{t} \cap \inhibpreset{T_2} = \emptyset$, we must have $\weights((p',t)) \geq \weights((t,p'))$, which implies $M''(p') \geq M'(p')$ and $t' \notin \en(M'')$.
	Therefore $t$ is safe in $M$.
\end{proof}

\section{Proof of Lemma~\ref{lemma:reach}}
\begin{proof}
	Assume that $M \not\models \varphi$.
	The proof proceeds by structural induction on $\varphi$.
	All cases, with the exception of $\varphi_1 \land \varphi_2$, are proved in Lemma 2 presented in~\cite{boenneland2018start}.
	\begin{description}
		\item $\varphi = \varphi_1 \land \varphi_2$:
		There are five subcases defined by Equation~\ref{eq:interest-and}:
		(1) $M\models\varphi_2$, (2) $M\models\varphi_1$, (3) $M\not\models\varphi_1$ and $\interest{M}{\varphi_1} \subseteq \safe{M}$, (4) $M\not\models\varphi_2$ and $\interest{M}{\varphi_2} \subseteq \safe{M}$, and (5) the default cases.
		\begin{itemize}
			\item Case (1): $M\models\varphi_2$:
			Since we have $M \not\models \varphi$ and $M\models\varphi_2$ we must therefore have that $M \not\models \varphi_1$ by the semantics of $\varphi$.
			By Equation~\ref{eq:interest-and}, since $M\models\varphi_2$, we have $\interest{M}{\varphi_1 \land \varphi_2} = \interest{M}{\varphi_1}$.
			By the induction hypothesis this implies $M' \not\models \varphi_1$, and from this and the semantics of $\varphi$ we have $M' \not\models\varphi$.
			\item Case (2): $M\models\varphi_1$:
			This case is symmetric to Case (1) and follows the same approach.
			\item Case (3): $M\not\models\varphi_1$ and $\interest{M}{\varphi_1} \subseteq \safe{M}$:
			By Equation~\ref{eq:interest-and} we have $\interest{M}{\varphi_1 \land \varphi_2} = \interest{M}{\varphi_1}$.
			By the induction hypothesis this implies $M' \not\models \varphi_1$, and from this and the semantics of $\varphi$ we have $M' \not\models\varphi$.
			\item Case (4): $M\not\models\varphi_2$ and $\interest{M}{\varphi_2} \subseteq \safe{M}$:
			This case is symmetric to Case (3) and follows the same approach.
			\item Case (5): Default:
			Since we have $M \not\models \varphi$ we know there exists $i \in \{1,2\}$ s.t. $M \not\models \varphi_i$ by the semantics of $\varphi$.
			By Equation~\ref{eq:interest-and} we have $\interest{M}{\varphi_1 \land \varphi_2} = \interest{M}{\varphi_1} \cup \interest{M}{\varphi_2}$.
			By the induction hypothesis this implies $M' \not\models \varphi_i$, and from this and the semantics of $\varphi$ we have $M' \not\models\varphi$.
		\end{itemize}
	\end{description}
\end{proof}

\section{Proof of Lemma~\ref{lemma:cycle}}
\begin{proof}
	\textit{Termination}:
	Since $\transitions$ is finite the loop in line~\ref{line:inf-transition-trivial} can iterate a finite number of times and it terminates.
	It is clear that the sets $\markedp$ and $\freshp$ are only increasing in the while-loop in line~\ref{line:place-marked-1}, and terminates if they ever become equal.
	Since these sets are only increasing, and $\places$ is finite, the while-loop can iterate at most finite times and it terminates.
	Since $\transitions$ is finite the loop in line~\ref{line:inf-transition} can iterate a finite number of times and it terminates.

	\textit{Correctness}:
	The trivial case where there exists $t \in \transitions_2$ s.t. $\preset{t} = \emptyset$ is handled in line~\ref{line:inf-transition-trivial}.

	Assume that there exists $w \in \transitions_2^{\omega}$ s.t. $M \rtrans[w]$ and there exists $t \in \transitions_2$ that occurs infinitely often in $w$.
	If $w$ is fireable in $M$ with inhibitor arcs then it is also fireable in $M$ without inhibitor arcs, i.e. removing inhibitor arcs does not remove paths.
	As an overapproximation we assume that all inhibitor arcs in the algorithm have a weight of $\infty$.

	It follows from that $t$ occurs infinitely often in $w$ that $v,u \in \transitions^*$ s.t. $M \rtrans[v] M' \rtrans[tu] M''$, $vtu$ is a prefix of $w$, and for all $p \in \preset{t}$ we have $M'(p) \leq M''(p)$, otherwise $p$ will eventually lack a sufficient number of tokens.

	First we want to show that $t \in \infinitef$.
	Assume for the sake of contradiction that $t \in \finitef$.
	Then there exists $p \in \preset{t}$ s.t. $p \in \finitef$ and $t$ cannot occur infinitely often in $w$ since $p$ cannot provide enough tokens, a contradiction.
	Therefore, we have $\preset{t} \subseteq \infinitef$, $t \notin \finitef$, and $t \in \infinitef$.

	Next we want to show that $\preset{t} \subseteq \markedp$.
	Let $P_0 = \{ p \in \places \mid M(p) > 0 \}$ and for all $i \geq 1$ we have $P_i = \{ p \in \places \mid p \in P_{i-1} \lor \exists t \in \transitions_2.\ p \in \preset{t} \land \preset{t} \subseteq P_{i-1} \}$.
	For all $j \geq 1$ we have $P_{j-1} \subseteq P_j$.
	Because $\places$ is finite we have that there exists $i \geq 1$ s.t. for all $i < j$ we have $P_i = P_j$, and $P_i = \markedp$ after the loop in line~\ref{line:place-marked-1} terminates.
	Intuitively, $P_i$ is an overapproximation of all places that can be marked by $1$ or more tokens at any intermediate marking by firing player $2$ transitions from $M$.
	For all $p \in \preset{t}$ if $M(p) > 0$ then $p \in P_0$ and also $p \in P_i$.
	If $M(p) < 1$ then we can infer that there exists $t' \in \transitions_2$ that occurs in $v$ and $p \in \postset{t'}$, otherwise we would not have $t \in \en(M')$.
	Therefore we must have $\preset{t} \subseteq P_i$ since $P_i$ is an overapproximation.

	We have shown $t \in \infinitef$ and $\preset{t} \subseteq \markedp$, and from line~\ref{line:add-t} we have $t \in \mathit{cycle}(N,M)$.
\end{proof}

\section{Proof of Theorem~\ref{prop:turn-game-preservation}}
\begin{proof}
	We shall argue that any reduction $\reduction$ satisfying the conditions of the theorem also satisfies the~\ref{rule:stub-init},~\ref{rule:stub},~\ref{rule:reach},~\ref{rule:game-1},~\ref{rule:game-2},~\ref{rule:safe},~\ref{rule:cycle}, and~\ref{rule:dead} conditions.
	\begin{itemize}
		\item (\ref{rule:stub-init}):
		Follows from Condition~\ref{item:contested}.
		\item (\ref{rule:stub}):
		Let $M,M' \in \markings$ be markings, $t \in \reduction(M)$, and $w \in \overline{\reduction(M)}^*$.
		We will show that if $M \rtrans[wt] M'$ then $M \rtrans[tw] M'$.

    		Let $M_w \in \mathcal{M}(N)$ be a marking s.t. $M \rtrans[w] M_w$.
		Assume for the sake of contradiction that $t \notin \en(M)$.
		Then $t$ is disabled in $M$ there is $p \in \preset{t}$ such that $M(p) < \weights((p,t))$ or there is $p \in \inhibpreset{t}$ such that $M(p) \geq \inhib((p,t))$.
		In the first case, due to Condition~\ref{item:disabled-1} all the transitions that can add tokens to $p$ are included in $\reduction(M)$.
		Since $w \in \overline{\reduction(M)}^*$ this implies that $M_w(p) < \weights((p,t))$ and $t \notin \en(M_w)$ contradicting our assumption that $M_w \rtrans[t] M'$.
		In the first case, due to Condition~\ref{item:disabled-2} all the transitions that can remove tokens from $p$ are included in $\reduction(M)$.
		Since $w \in \overline{\reduction(M)}^*$ this implies that $M_w(p) \geq \inhib((p,t))$ and $t \notin \en(M_w)$ contradicting our assumption that $M_w \rtrans[t] M'$.
		Therefore we must have that $t \in \en(M)$.

		Since $t \in \en(M)$ there is $M_t \in \markings$ s.t. $M \rtrans[t] M_t$.
		We have to show that $M_t \rtrans[w] M'$ is possible.
 		For the sake of contradiction, assume that this is not the case.
		Then there must exist a transition $t'$ that occurs in $w$ that became disabled because $t$ was fired.
		There are two cases: $t$ removed one or more tokens from a shared pre-place $p \in \predecr{t} \cap \preset{t'}$ or added one or more tokens to a place $p \in \postincr{t} \cap \inhibpreset{t'}$.
		In the first case, due to Condition~\ref{item:enabled-1} all the transitions that can remove tokens from $p$ are included in $\reduction(M)$, implying that $t' \in \reduction(M)$.
		Since $w \in \overline{\reduction(M)}^*$ such a $t'$ cannot exist.
		In the second case, due to Condition~\ref{item:enabled-2} all the transitions that can add tokens to $p$ are included in $\reduction(M)$, implying that $t' \in \reduction(M)$.
		Since $w \in \overline{\reduction(M)}^*$ such a $t'$ cannot exist.
		Therefore we must have that $M_t \rtrans[w] M'$ and we can conclude with $M \rtrans[tw] M'$.
    		%We note here that the execution sequences $wt$ and $tw$ must lead to the same marking as the order of transition firings does not impact the reachable marking.
		\item (\ref{rule:reach}):
		Follows from Condition~\ref{item:interesting} and Lemma~\ref{lemma:reach}.
		\item (\ref{rule:game-1}):
		Let $M \in \markings$ be a marking and $w \in \overline{\reduction(M)}^*$ s.t. $M \rtrans[w] M'$.
		We will show that if $\en_2(M) = \emptyset$ then $\en_2(M') = \emptyset$.

		Assume that $\en_2(M) = \emptyset$.
		Then by Condition~\ref{item:opponent-2} we have $\transitions_2 \subseteq \reduction(M)$.
		Let $t \in \transitions_2$ be a player $2$ transition.
		By Condition~\ref{item:prop-disabled} we know that either: There exists $p \in \preset{t}$ s.t. $M(p) < \weights((p,t))$ and $\preincr{p} \subseteq \reduction(s)$, or there exists $p \in \inhibpreset{t}$ s.t. $M(p) \geq \inhib((p,t))$ and $\postdecr{p} \subseteq \reduction(s)$.
		In the first case, in order to enable $t$ at least one transition from $\preincr{p}$ has to be fired.
		However, we know $\preincr{p} \subseteq \reduction(s)$ is true, and therefore none of the transitions in $\preincr{p}$ can occur in $w$, which implies $t \notin \en_2(M')$.
		In the second case, in order to enable $t$ at least one transition from $\postdecr{p}$ has to be fired.
		However, we know $\postdecr{p} \subseteq \reduction(s)$ is true, and therefore none of the transitions in $\postdecr{p}$ can occur in $w$, which implies $t \notin \en_2(M')$.
		These two cases together implies $\en_2(M') = \emptyset$.
		\item (\ref{rule:game-2}):
		Follows the same approach as~\ref{rule:game-1}.
		\item (\ref{rule:safe}):
		Follows from Condition~\ref{item:safe}.
		\item (\ref{rule:cycle}):
		Follows from Condition~\ref{item:cycle} and Lemma~\ref{lemma:cycle}.
		\item (\ref{rule:dead}):
		Let $M \in \markings$ be a marking and $w \in \overline{\reduction(M)}^*$ s.t. $M \rtrans[w] M'$.
		We will show that if $\en_2(M) \neq \emptyset$ then there exists $t \in \en_2(M) \cup \reduction(M)$ s.t. $t \in \en_2(M')$.

		Assume that $\en_2(M) \neq \emptyset$.
		From Condition~\ref{item:deadlock} we know that there exists $t \in \en_2(M) \cup \reduction(M)$ s.t. $\postdecr{(\preset{t})} \cup \preincr{(\inhibpreset{t})} \subseteq \reduction(M)$.
		Assume for the sake of contradiction that $t \notin \en_2(M')$.
		In this case there must either exist $p \in \preset{t}$ s.t. $M'(p) < \weights((p,t))$, or there exists $p \in \inhibpreset{t}$ s.t. $M'(p) \geq \inhib((p,t))$.
		In the first case, since $t \in \en_2(M)$ we have that $M(p) \geq  \weights((p,t))$.
		Therefore at least one transition from $\postdecr{p}$ has to have been fired.
		However, we know $\postdecr{(\preset{t})} \subseteq \reduction(M)$ is true, and therefore none of the transitions in $\postdecr{p}$ can occur in $w$, which implies $M'(p) \geq  \weights((p,t))$, a contradiction.
		In the second case, since $t \in \en_2(M)$ we have have that $M(p) < \inhib((p,t))$.
		Therefore at least one transition from $\preincr{p}$ has to have been fired.
		However, we know $\preincr{(\preset{t})} \subseteq \reduction(M)$ is true, and therefore none of the transitions in $\preincr{p}$ can occur in $w$, which implies $M'(p) < \inhib((p,t))$, a contradiction.
		Therefore $t \notin \en_2(M')$ cannot be true, and we must have that $t \in \en_2(M')$.
	\end{itemize}
	This completes the proof of the theorem.
\end{proof}

\section{Proof of Theorem~\ref{thm:alg}}
\begin{proof}
	\textit{Termination}: If $\en_1(M) \neq \emptyset$ and $\en_2(M) \neq \emptyset$ then we terminate in line~\ref{line:mixed}.
	Otherwise $Y \neq \emptyset$ and we enter the while-loop in Algorithm~\ref{alg:saturation-2}.
	Notice that $X \cap Y = \emptyset$ is always the case in the execution of Algorithm~\ref{alg:saturation-2}.
	We never remove transitions from $X$ after they have been added.
	Therefore, since in line~\ref{line:retire} of Algorithm~\ref{alg:saturation-2} a new transition is added to $X$ at the end of each loop iteration, the loop can iterate at most once for each transition.
	Since $T$ is finite by the Petri Net Game definition, the loop iterates a finite number of times, and Algorithm~\ref{alg:saturation-2} terminates.
	If $\en_1(M) \cap X \nsubseteq \safe{M}$ then we terminate in line~\ref{line:safe} of Algorithm~\ref{alg:saturation}, and otherwise we return in line~\ref{line:final-return} and Algorithm~\ref{alg:saturation} terminates.

	\textit{Correctness}: It was shown that the construction in Theorem~\ref{prop:turn-game-preservation} results in a set that is a stubborn set of a stable reduction.
	 It is therefore sufficient to show that Algorithm~\ref{alg:saturation} replicates the construction.
	 Notice that every transition that is added to $Y$ is eventually added to $X$ in line~\ref{line:retire} and returned in line~\ref{line:final-return} of Algorithm~\ref{alg:saturation-2}.
	 Let $t \in Y$.

	 Condition~\ref{item:contested}: If $\en_1(M) \neq \emptyset$ and $\en_2(M) \neq \emptyset$ then we return $\transitions$ in line~\ref{line:mixed} of Algorithm~\ref{alg:saturation}.

	 Condition~\ref{item:safe}: If $\en_1(M) \cap \reduction(M) \nsubseteq \safe{M}$ then we return $\transitions$ in line~\ref{line:safe} of Algorithm~\ref{alg:saturation}.

	 Condition~\ref{item:interesting}: We have $\interest{M}{\varphi} \subseteq Y$ in line~\ref{line:interesting} of Algorithm~\ref{alg:saturation}.

	 Condition~\ref{item:opponent-1}: We have $\transitions_1 \subseteq Y$ in line~\ref{line:p1} of Algorithm~\ref{alg:saturation}.

	 Condition~\ref{item:opponent-2}: We have $\transitions_2 \subseteq Y$ in line~\ref{line:p2} of Algorithm~\ref{alg:saturation}.

	 Condition~\ref{item:cycle}: We have $\mathit{cycle}(N,M) \subseteq Y$ in line~\ref{line:cycle} of Algorithm~\ref{alg:saturation}.

	 Condition~\ref{item:disabled-1}: In line~\ref{line:pick-dis-1} we pick any $p \in \preset{t}$ s.t. $M(p) < \weights((p,t))$, and in line~\ref{line:dis-1-add} of Algorithm~\ref{alg:saturation-2} we add $\preincr{p}$ to $Y$.

	 Condition~\ref{item:disabled-2}: In line~\ref{line:pick-dis-2} we pick any $p \in \inhibpreset{t}$ s.t. $M(p) \geq \inhib((p,t))$, and in line~\ref{line:dis-2-add} of Algorithm~\ref{alg:saturation-2} we add $\postdecr{p}$ to $Y$.

	 Condition~\ref{item:enabled-1}: In line~\ref{line:enabled} of Algorithm~\ref{alg:saturation-2} we add $\postset{(\predecr{t})}$ to $Y$.

	 Condition~\ref{item:enabled-2}: In line~\ref{line:enabled} of Algorithm~\ref{alg:saturation-2} we add $\inhibpostset{(\postincr{t})}$ to $Y$.

	 Condition~\ref{item:deadlock}: In line~\ref{line:dead-pick} of Algorithm~\ref{alg:saturation} we pick any $t' \in \en_2(M)$ and in line~\ref{line:p1} we add $\postdecr{(\preset{t})} \cup \preincr{(\inhibpreset{t})}$ to $Y$.
\end{proof}
